# Supplementary material for: Adaptive Importance Sampling based Neural Network framework for Reliability and Sensitivity Prediction for Variable Stiffness Composite Laminates with hybrid uncertainties
Source: arXiv:2001.09884 source file (2020-01-27)
Supplement: Supplementary file 1 [file AppendixA.tex]

%\begin{appendices} 

By inserting the strain-displacement relationship (Eq. \ref{eqn:32}) in Equations \ref{eq:520} and \ref{eq:521}, one obtains the following: 

\begin{equation}
   \begin{split} 
   E_{d} &= \frac{1}{2} \int_{xy} \bigg( A_{11} \left(\frac{\partial u_{0}}{\partial x}\right)^2 + A_{22} \left(\frac{\partial v_{0}}{\partial y}\right)^2 + 2 A_{12} \left(\frac{\partial u_0}{\partial x} \frac{\partial v_0}{\partial y} \right) + A_{33} \left(\frac{\partial u_0}{\partial y} \right)^2  dxdy\\
    & + \left(\frac{\partial v_0}{\partial x}\right)^2 + 2\left(\frac{\partial u_0}{\partial y} \frac{\partial v_0}{\partial x} \right) + 2A_{13} \left[ \left( \frac{\partial u_0}{\partial x} \frac{\partial u_0}{\partial y} \right) + \left(\frac{\partial u_0}{\partial x} \frac{\partial v_0}{\partial x} \right) \right] \\
    &+ 2A_{23} \left[ \left( \frac{\partial v_0}{\partial y} \frac{\partial u_0}{\partial y} \right) + \left(\frac{\partial v_0}{\partial y} \frac{\partial v_0}{\partial x} \right) \right] + 2 B_{11} \left( \frac{\partial u_0}{\partial x} \frac{\partial \beta_x}{\partial x} \right) + 2 B_{22} \left( \frac{\partial v_0}{\partial y} \frac{\partial \beta_y}{\partial y} \right) \\ 
    &+ 2 B_{12} \left( \frac{\partial u_0}{\partial x} \frac{\partial \beta_y}{\partial y} \right) + \left( \frac{\partial v_0}{\partial y} \frac{\partial \beta_x}{\partial x} \right) \\ 
    &+ 2 B_{33} \left[ \left( \frac{\partial u_0}{\partial y} \frac{\partial \beta_x}{\partial y} \right) + \left( \frac{\partial u_0}{\partial y} \frac{\partial \beta_y}{\partial x} \right) + \left( \frac{\partial v_0}{\partial x} \frac{\partial \beta_x}{\partial y} \right) + \left( \frac{\partial v_0}{\partial x} \frac{\partial \beta_y}{\partial x} \right) \right] \\ 
    &+ 2 B_{13} \left[ \left( \frac{\partial u_0}{\partial y} \frac{\partial \beta_x}{\partial x} \right) + \left( \frac{\partial v_0}{\partial x} \frac{\partial \beta_x}{\partial x} \right) + \left( \frac{\partial u_0}{\partial x} \frac{\partial \beta_x}{\partial y} \right) + \left( \frac{\partial u_0}{\partial x} \frac{\partial \beta_y}{\partial x} \right) \right] \\ 
    &+ 2 B_{23} \left[ \left( \frac{\partial u_0}{\partial y} \frac{\partial \beta_y}{\partial y} \right) + \left( \frac{\partial v_0}{\partial x} \frac{\partial \beta_y}{\partial y} \right) + \left( \frac{\partial v_0}{\partial y} \frac{\partial \beta_x}{\partial y} \right) + \left( \frac{\partial v_0}{\partial y} \frac{\partial \beta_y}{\partial x} \right) \right] \\ 
    &+ D_{11} \left( \frac{\partial \beta_x}{\partial x}  \right)^2 + D_{22} \left( \frac{\partial \beta_y}{\partial y}\right)^2 + 2 D_{12} \left( \frac{\partial \beta_x}{\partial x} \frac{\partial \beta_y}{\partial x} \right)+ D_{33} \left( \frac{\partial \beta_x}{\partial y}\right)^2\\ &+ \left( \frac{\partial \beta_y}{\partial x}  \right)^2 + 2 \left( \frac{\partial \beta_x}{\partial y} \frac{\partial \beta_y}{\partial x}  \right) + 2 D_{13} \left[ \left( \frac{\partial \beta_x}{\partial x} \frac{\partial \beta_x}{\partial y} \right) + \left( \frac{\partial \beta_x}{\partial x} \frac{\partial \beta_y}{\partial x} \right) \right] \\ 
    &+ 2 D_{23} \left[ \left( \frac{\partial \beta_y}{\partial y} \frac{\partial \beta_x}{\partial y} \right) + \left( \frac{\partial \beta_y}{\partial y} \frac{\partial \beta_y}{\partial x} \right) \right] + k_s \bigg( A_{44} \left(\frac{\partial w_0}{\partial x} \right)^2 + A_{55} \left( \frac{\partial w_0}{\partial y}\right)^2 \\ 
    &+ 2 A_{45} \left(\frac{\partial w_0}{\partial x} \frac{\partial w_0}{\partial y} \right) + A_{44} (\beta_x)^2 + A_{55} (\beta_y)^2 + 2 A_{44} \left( \frac{\partial w_0}{\partial x} \beta_x \right) + 2A_{55} \left( \frac{\partial w_0}{\partial y} \beta_y \right) \\
    &+ 2 A_{45} \beta_x \beta_y \bigg)\bigg) dxdy
    \end{split}
\end{equation}

\noindent where 

\begin{align}
    A_{ij}(x) &= \sum_{k=1}^{NL} \int_{h_k}^{h_{k+1}} \left[ \overline{Q}_{ij}^k \right] dz  \\ 
    B_{ij}(x) &= \sum_{k=1}^{NL} \int_{h_k}^{h_{k+1}} \left[ \overline{Q}_{ij}^k \right] z dz \\ 
    D_{ij}(x) &= \sum_{k=1}^{NL} \int_{h_k}^{h_{k+1}} \left[ \overline{Q}_{ij}^k \right] z^2 dz
\end{align}

\noindent and 

\begin{equation}
    \begin{split}
        E_c &= \frac{1}{2} \int_{xy} \bigg[  \rho_A \left( \frac{\partial u_0}{\partial t} \right)^2 +  \rho_A \left( \frac{\partial v_0}{\partial t} \right)^2 +  \rho_A \left( \frac{\partial w_0}{\partial t} \right)^2 +  \\ 
        &+ 2 \rho_B \left[ \left( \frac{\partial u_0}{\partial t} \frac{\partial \beta_x}{\partial t} \right) + \left( \frac{\partial v_0}{\partial t} \frac{\partial \beta_y}{\partial t} \right) \right] \\ 
        &+ \rho_D \left( \frac{\partial \beta_x}{\partial t} \right)^2 + \rho_D \left( \frac{\partial \beta_y}{\partial t} \right)^2  \bigg] dxdy
    \end{split}
\end{equation}

\noindent Here, $NL$ stands for the number of plies in the lamina.

%\end{appendices}
